# Supplementary material for: Mitigating Test-Time Bias for Fair Image Retrieval
Source: arXiv:2305.19329 source file (2023-05-23)
Supplement: Supplementary file 1 [file additional_analysis.tex]

\documentclass{article}

\begin{document}

\section{Additional Analysis Results}
%logistic regression model S -> probability of g

Here we provide extended analysis support our Section~\ref{sec: fair_analysis}.

The relationship between bias and

Apart from the image retrieval task loss Ltask\mathcal{L}_{\text{task}}, learning gθg_{\theta} often involves incorporating strategies to reduce biases, ensuring more fair outputs from the algorithm.
% another fairness loss Lfairness\mathcal{L}_{\text{fairness}} is usually added to reduce the bias in the output
\rh{where and by whom?}.
%
% \[
% \mathcal{L}(V_K, c) = \mathcal{L}_{\text{task}}(V_K, c) + \lambda \mathcal{L}_{\text{fairness}}(V_K).
% \]
%
\rh{and λ\lambda is?}
In this section, we take the goal to reduce gender bias as a case study.  Adversarial training is employed by \citet{edwards2015censoring, berg2022prompt, xu2021robust}, in order to minimize the image-text encoders' ability to provide useful information to the adversary, where the adversary is a classifier that is specifically designed to distinguish between biological sexes (male, female) based on the output of image-text encoders. Thus, with adversarial learning, the learned representation of image-text encoders is less biased and more fair with respect to the biological sexes. \citet{wang2021gender} uses mutual information(MI) minimization, which mitigates bias by reducing the dependence between the learned features from fϕ(v)f_{\phi}(v) and fψ(c)f_{\psi}(c) and biological sexes AA. 
\rh{this makes no sense, they use adversarial, MI and neutralization to do what? how?}. The shared objective \rh{which shared objective?} of these approaches is to make the text-image representation (fϕ(v),fψ(c))(f_\phi(v), f_\psi(c)) independent of gender attributes AA.
However, we demonstrate that such independence is not sufficient to eliminate the bias B(VK)B(V_K) in image retrieval in the following analysis.  \shuai{Formula and more explanations about their idea here.}
\rh{why do you need the equation below?}
% \[
% f_\phi(v) \perp A 
% \]
% However, we show that such mutual information does not help reduce gender bias. Specifically, setting the mutual information between ... 
%as zero indicates that the gender of each vi∈Vv_i\in V is independent of ... \rh{?} 
For query cc, suppose the ratio of male images among all relevant images in the dataset is
\[
\alpha(c) = \frac{\left|\{v \mid f(v)=c \ \text{and}\  A(v)=+1\}\right|}{\left|\{v \mid f(v)=c\}\right|}.
\]
For a bag of correct retrieval VK={v1,v2,⋯vK}V_K=\{v_1, v_2, \cdots v_K\}, since its gender is independent from ... \rh{?}, every viv_i has α(c)\alpha(c) probability to be male, and their genders are independent from each other.
Thus, the number of male images among VKV_K conforms to binomial distribution m∼Binom(K,α(c))m\sim \text{Binom}(K, \alpha(c)).  and the expected gender bias can be computed as \rh{stopped here, it is becoming difficult to follow.}
\[
\mathbb{E}[B(V_K)] = \sum_{m=0}^K \binom{K}{m} [\alpha(c)]^m [1-\alpha(c)]^{K-m} \cdot \frac{|K-2m|}{K},
\]
which is always positive for any meaningful KK. In Figure~?????????\ref{fig: binom}, we visualize the relationship between bias B(VK)B(V_K) and the positive attribute ratio α(c)\alpha(c), as well as the bag size KK. In the left subplot, despite the dataset being balanced, meaning that α(c)=0.5\alpha(c)=0.5, the bias still does not desirably close to 00 unless selecting a considerably large bag size K>200K > 200.  From the left subplot, we observe that bias is predominantly influenced by α(c)\alpha(c), with a rapid increase observed when α(c)>0.6\alpha(c) > 0.6 or α(c)<0.4\alpha(c) < 0.4, which very commonly happens in dataset such as COCO-2014~\cite{zhao2021understanding} and Occupations~\cite{kay2015unequal, celis2020implicit}, as shown in Table~?????????\ref{table: alpha}. In our experiment result, we include "random selection" as baseline to show the best of mutual information minimization can do for reducing bias. \shuai{just "positive" is too weak. Maybe draw a figure to show the bias can be large for larger KK.}
By analyzing retrieval results with varying mutual information, we calculate the average bias, B(V20)B(V_{20})
, and average similarity of images within a 20-image sliding window. A linear regression, y=ax+by=ax+b
, is fitted to demonstrate how the model's retrieval decisions are influenced by gender. Traditional methods strive to eradicate bias in the model's choices by bringing the slope aa
, closer to zero. However, due to the unbalanced nature of the source dataset (male:female  ≠1:1\neq 1:1), dataset bias persists (represented by intercept bb), resulting in biased retrieval outcomes even when the model is gender-blind. Our approach tackles both model and dataset biases, aiming to B(V20)B(V_{20})
, and average similarity of images within a 20-image sliding window. A linear regression, y=ax+by=ax+b
, is fitted to demonstrate how the model's retrieval decisions are influenced by gender. Existing methods strive to eradicate bias of model decision by forcing the model blind to the gender, meaning the slope is reduced to 00. However, due to the unbalanced nature of the source dataset (male:female ≠1:1\neq 1:1), dataset bias persists (represented by intercept bb
), resulting in biased retrieval outcomes even when the model is gender-blind. Our approach tackles both model and dataset biases simultaneously.

\begin{table}[!htb]
\centering
\caption{Average male ratio α\alpha across some popular datasets. Even the UTKface and FairFace are balanced, there is still a bias in gender representation.}
\begin{tabular}{llllll}
\hline
             & COCO-val & Occupation 1& Occupation 2 &  UTKFace & FairFace \\ \hline
Male ratio α\alpha  & 0.69 & 0.61     & 0.58 &  0.52    & 0.53     \\ \hline
\end{tabular}
\label{table: alpha}
\end{table}

\begin{figure}[!htb]
    \centering
\includegraphics[width=1.0\textwidth]{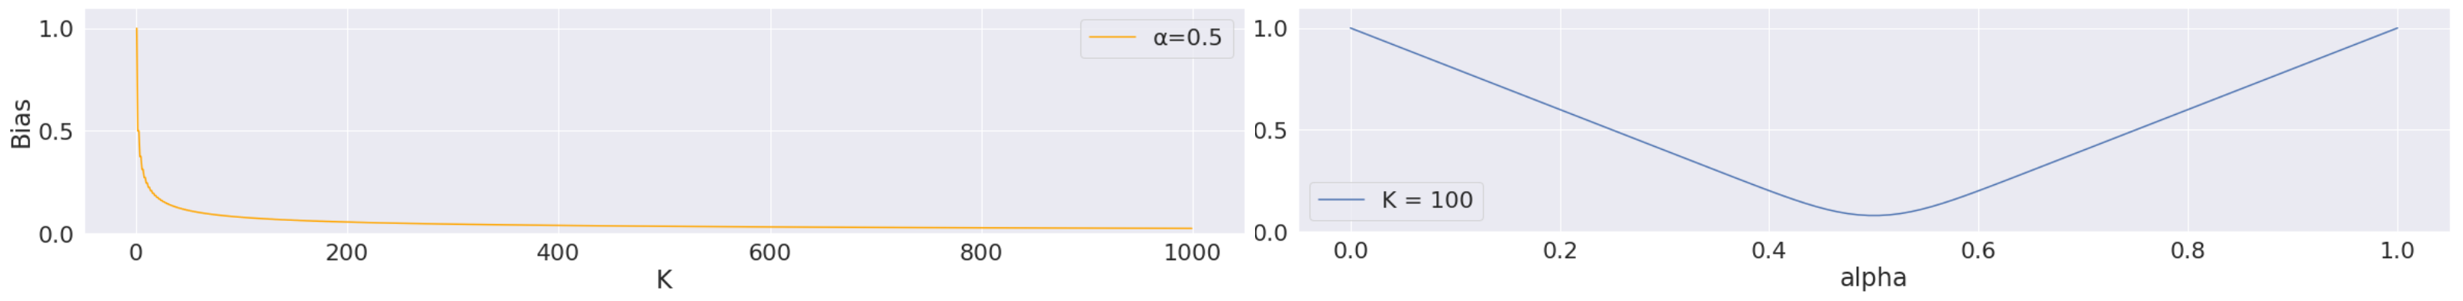}
    \caption{Expectation of bias B(VK)B(V_K) when representation and gender attributes are independent. Right: we illustrate the bias as a function of bag size KK, with α(c)=0.5\alpha(c) = 0.5; left: we depicts the relationship between bias and varying α(c)\alpha(c) for a fixed K=100K=100.
    
    }
    \label{fig: binom}
\end{figure}
\section{Debiasing as Structured Probabilistic Model.} \label{sec: fair_post_processing}\cite{goodfellow2016structured} 

To achieve gender-neutral query can stably produce neutral results in image-search models, we formulate the gender-neutral query as a constrained structure prediction problem, inspired by \cite{jiang2022constraint}:
\begin{equation}
    \begin{split}
          & p_(V_K| c) \begin{cases} 
\; > 0,  & \text{if}\; B(V_K) = \text{mod}(K, 2) \\ 
\; = 0, & \text{if}\; B(V_K) \neq \text{mod}(K, 2) 
\end{cases} ,
    \end{split}
\end{equation}
In our structured probabilistic model, we ensure that only the VKV_K satisfying to the fairness constraint are allowed to exist. Then, the expected bias B(VK)B(V_K) is,
\begin{equation}
\begin{split}
  & \mathbbm{E}[B(V_K)] = \sum |\sum_{v\in V_K} A(v)|p(V_K|c) = \text{mod}(K,2)
\end{split}
\end{equation}
The above deviation shows that our structured probabilistic model is able to consistently adheres to fairness constraint . Then, we introduce how to model our p(VK|c)p(V_K|c).

Instead of modeling the probability pθ(VK|c)p_{\theta}(V_K| c) directly, the model introduces an additional random variable zz and models it as a deterministic transformation from random variable zz and input variable cc to the output bag VKV_K.
Specifically, zz here can be interpreted as a decision variable to determine whether we should pick this image into our retrieval result based on its gender.
\begin{equation}
    \begin{split}
     & p_(V_K| c) = \int  p_(V_K| c, z)p(z)dz \\
     & p_(V_K| c, z) =\mathbbm{1}\{V_K =  f_{\theta}(c, z)\}
    \end{split} ,
\end{equation}
where we assume zz is from a known prior probability distribution p(z)p(z). In our case, zz is a variable of pre-assigned gender attribute to each image in the evaluation dataset, which can be annotated by users or predicted by a neural network. As a result, we only need to model pθ(VK|c,z)p_{\theta}(V_K|c, z) for the overall model. We further assume that pθ(VK|c,z)p_{\theta}(V_K|c, z) is a deterministic function. When pθ(VK|c,z)=1p_{\theta}(V_K|c, z)= 1, it indicates that the retrieved bag is considered being fair, and we choose to output it. On the other hand, if pθ(VK|c,z)=0p_{\theta}(V_K|c, z)= 0, we decide against selecting the unfair bag.  

Finding the function ff becomes quite simple when the dataset contains only male/female stereotypes. To achieve the least bias, we first divide the evaluation dataset into two groups consisting of only male and female images. Then, retrieve K/2K/2 pairs of images, with each pair containing one male and one female image from their respective groups. The expected bias output from our structured model becomes:
%However, when there are neutral images in the dataset, which means both a pair of male and female images satisfies the 
% Clearly, looking for a function that each time gives you a fair bag and maximizes the similarities between all images in the bag and the query cc is an NP-hard integer programming problem~\cite{celis2017ranking}.  For computationally efficient, we propose to formulate the fθf_{\theta} in a greedy way.  
% why subset...?
%
\begin{equation}
\begin{split}
    & B(V_K) = 
  \begin{cases} 
\; = B(\bigcup V_2) = \sum_{i=1}^{K/2} \frac{2}{K} B(V_2) = 0 ,  & \text{if KK is even.}  \\ 
\; B(V_1 \cup (\bigcup V_2)) = \frac{1}{K} + \sum_{i=1}^{(K-1)/2} \frac{2}{K-1} B(V_2) = \frac{1}{K} , & \text{if KK is odd.} 
\end{cases} ,
\end{split}
\end{equation}
PBM uses a simple greedy way to search for all qualified fair subsets of images related to query cc, and then aggregates them together.  

\section{Visual Debiasing Results on Real-world Web Image Search Data}

In Figureref{fig: vis_debias}, we exhibit a visualization of our debiasing result.
\begin{figure}[!htb]
    \centering
\includegraphics[width=1.\textwidth]{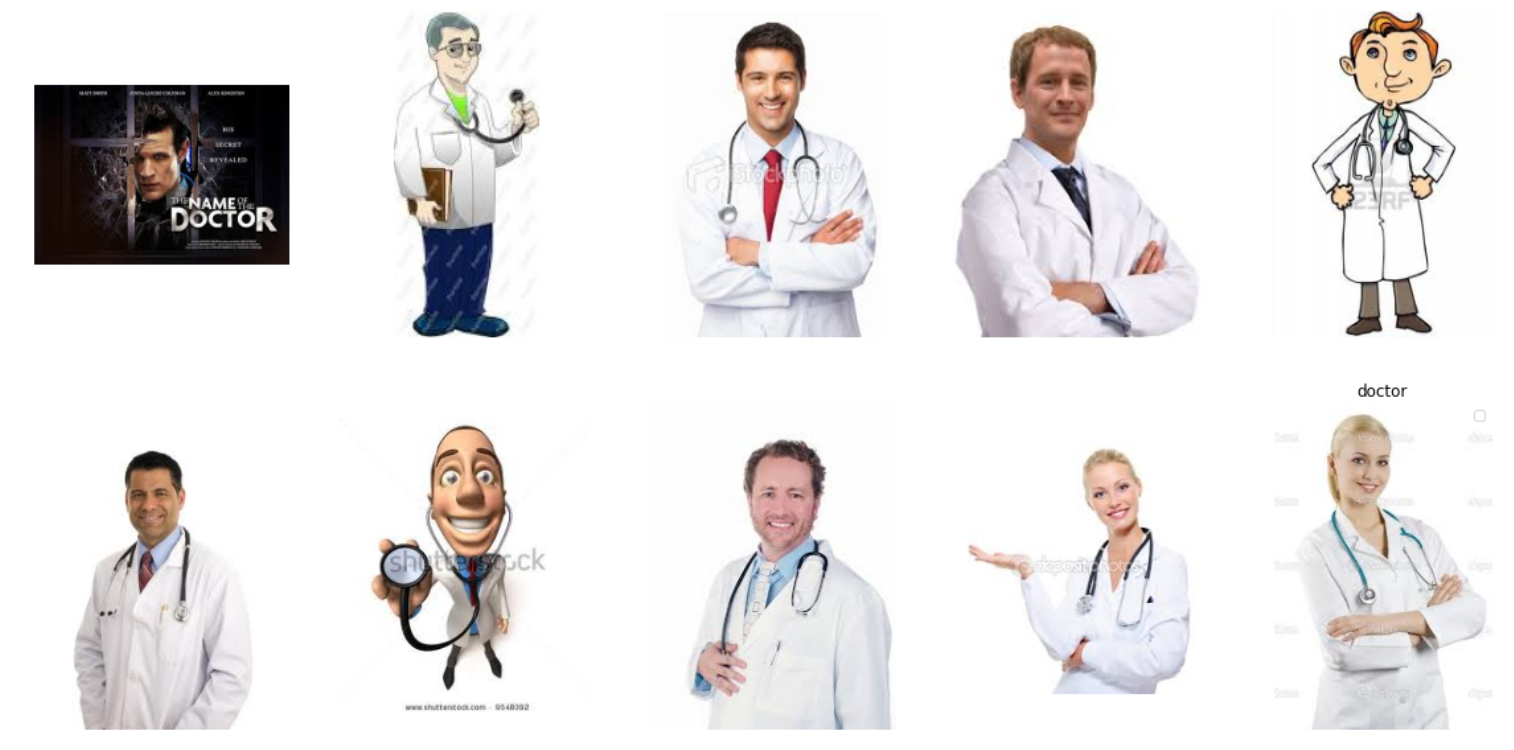}
\includegraphics[width=1.\textwidth]{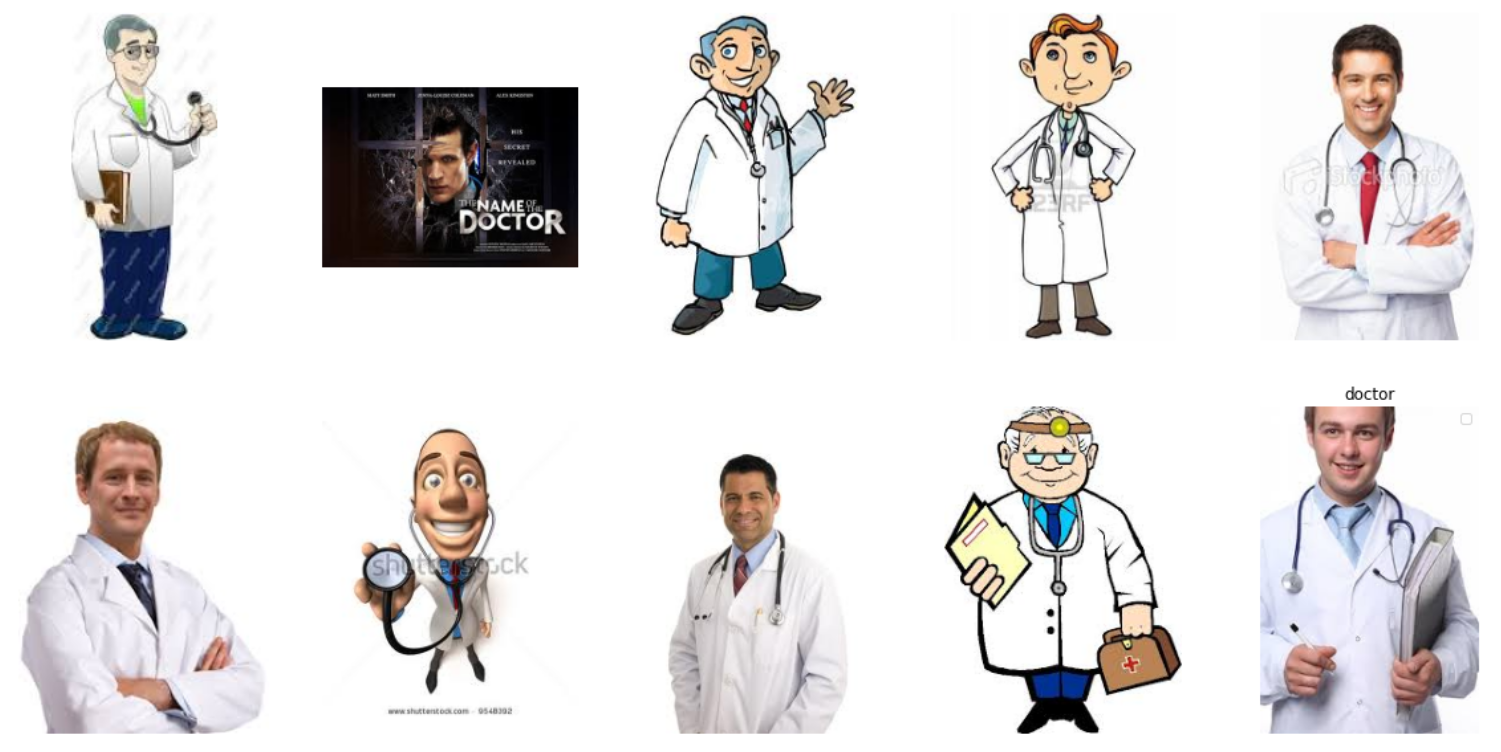}
\includegraphics[width=1.\textwidth]{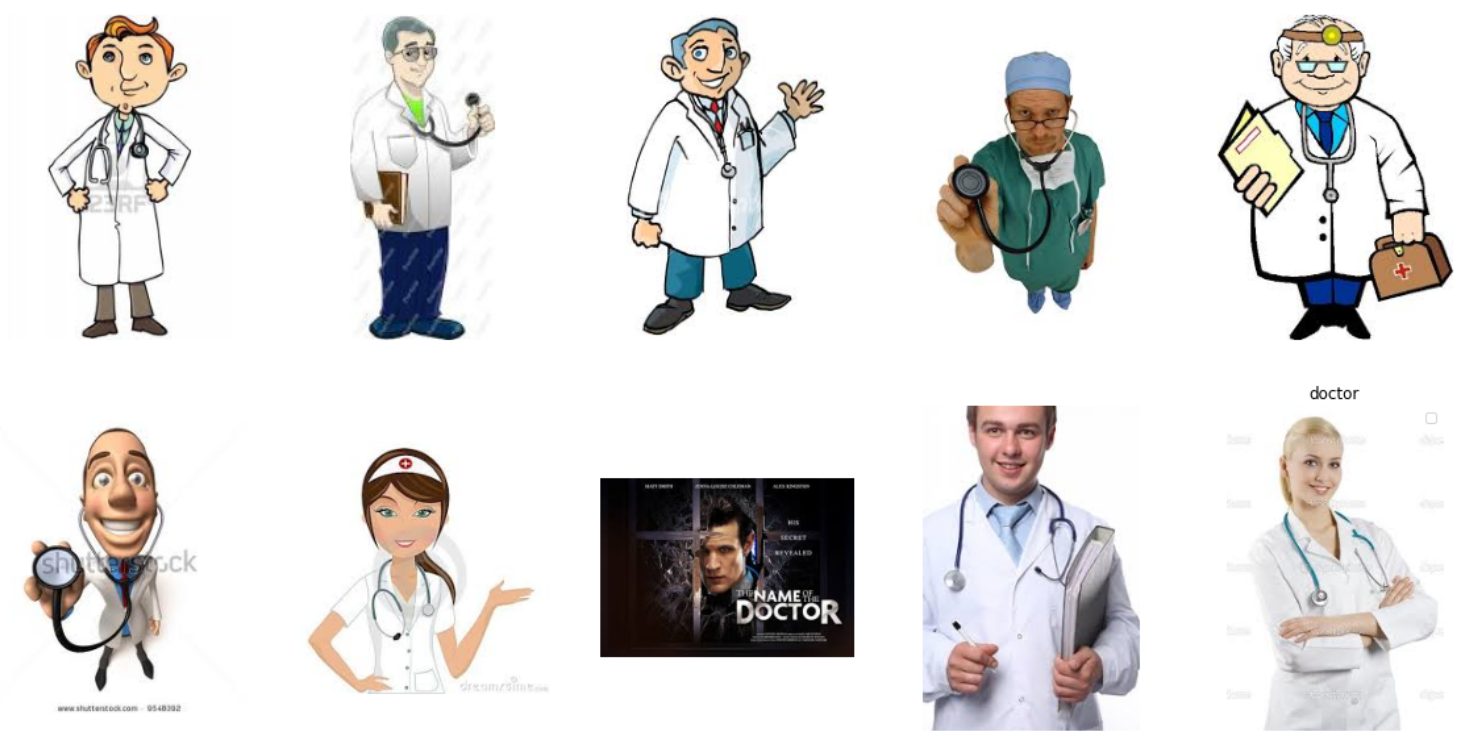}
\includegraphics[width=1.\textwidth]{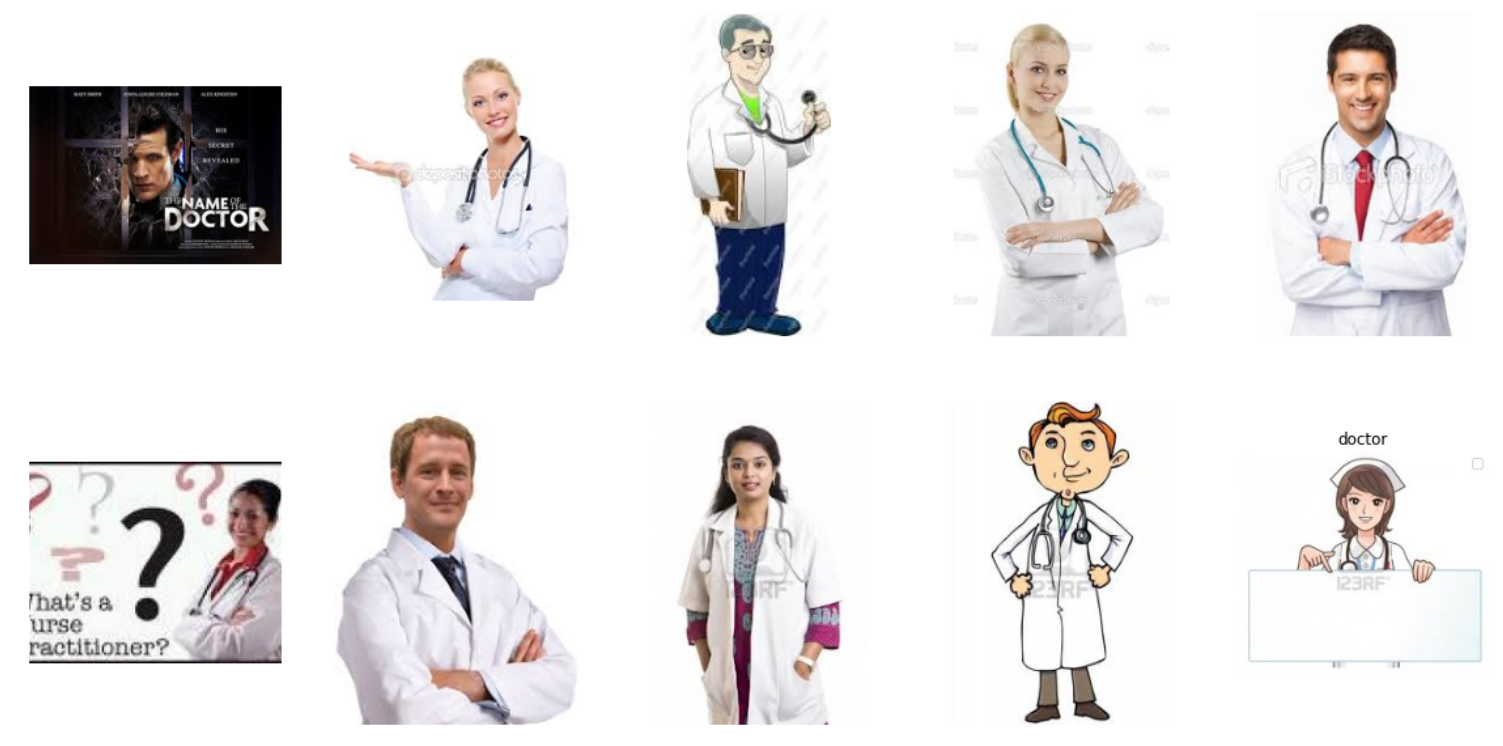}
    \caption{Visual Debiasing result on Occupation 1.}
    \label{fig: vis_debias}
\end{figure}

\end{document}
